# Supplementary material for: D-Flat: A Differentiable Flat-Optics Framework for End-to-End Metasurface Visual Sensor Design
Source: arXiv:2207.14780 source file (2022-08-08)
Supplement: Supplementary file 1 [file supplement_rendering_depth.tex]

% \begin{figure}%[h!]
%     \centering
%     \includegraphics[width=1.0\columnwidth]{appendix_figs/render.pdf}
%     \caption{caption}
%     \label{fig:occlusion}
% \end{figure}

\begin{figure}%[h!]
    \centering
    \includegraphics[width=1.0\columnwidth]{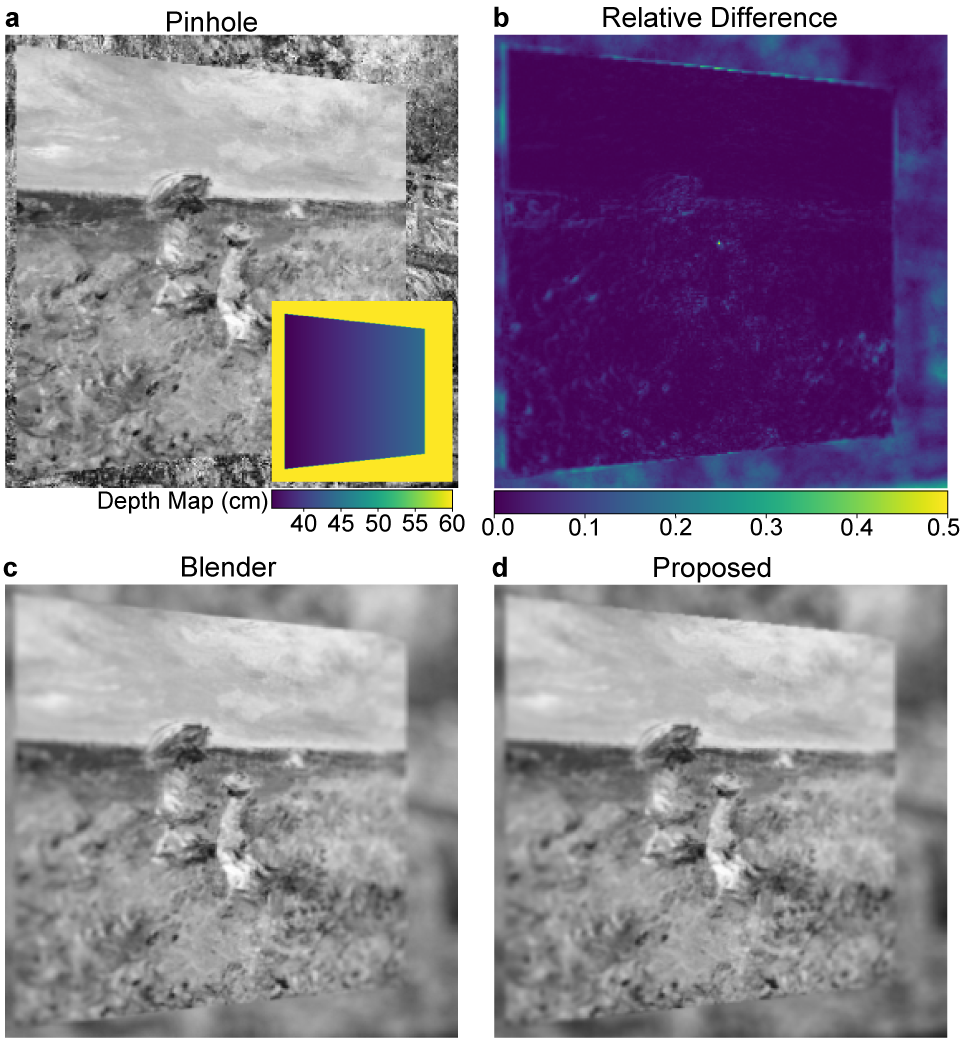}
    \caption{caption}
    \label{fig:depth_blender}
\end{figure}
